# Supplementary material for: Neural Fields for Fast and Scalable Interpolation of Geophysical Ocean Variables
Source: arXiv:2211.10444 source file (2022-11-18)
Supplement: Supplementary file 1 [file 8_appendix.tex]

\appendix

\section{Appendix}

\subsection{Optimal Interpolation}

This is a functional method which results in a conditional distribution which produces functions which can describe the data and draw samples which could potentially describe the underlying distribution given the training samples. Finally, we get a predictive mean and variance function which can produce mean and variance estimates conditioned on the observations.

\begin{equation}
    \boldsymbol{f} \sim \mathcal{GP}\left(\boldsymbol{m}_{\alpha}(\mathbf{x}_\phi), \boldsymbol{k_\alpha}(\mathbf{x}_\phi, \mathbf{x}_\phi')\right)
\end{equation}

\begin{align}
    \boldsymbol{\mu}(\mathbf{x}_\phi^*) &= \boldsymbol{m}(\mathbf{x}_\phi^*) + \boldsymbol{k}(\mathbf{X}_\phi,\mathbf{x}_\phi^*)\left(\mathbf{K}_{GP}+\sigma^2\mathbf{I} \right)^{-1}\left(y_{\text{obs}} - \boldsymbol{m}(\mathbf{x}_\phi)\right)
    % = \boldsymbol{k}(\mathbf{X}_\phi,\mathbf{x}_\phi^*)\boldsymbol{\alpha}
    \\
    \boldsymbol{\sigma}^2 (\mathbf{x}_\phi^*) &= \sigma^2 + \boldsymbol{k}(\mathbf{x}_\phi^*, \mathbf{x}_\phi^*) + \boldsymbol{k}(\mathbf{X}_\phi,\mathbf{x}_\phi^*)^\top\left(\mathbf{K}_\mathcal{GP}+\sigma^2\mathbf{I} \right) \boldsymbol{k}(\mathbf{X}_\phi,\mathbf{x}_\phi^*)
\end{align}

\subsection{Neural Fields}

\begin{equation}
    y_{\text{obs}} = \boldsymbol{f_\theta}(\mathbf{x}_\phi) + \epsilon
\end{equation}

Optionally include extra information (complete proofs, additional experiments and plots) in the appendix.
This section will often be part of the supplemental material.
